# Supplementary material for: ECCentric: An Empirical Analysis of Quantum Error Correction Codes
Source: arXiv:2511.01062 source file (2026-08-18)
Supplement: Supplementary file 1 [file background_ext.tex]

\section{Extended Background}
\label{sec:ext_background}
As described by Nielsen and Chuang~\cite{Nielsen_Chuang_2010}, in quantum computing, the basic unit of information is the \textit{qubit}. Unlike a classical bit, which exists exclusively in one of two states, a qubit can reside in a quantum superposition of basis states, representing both simultaneously. Quantum operations, known as \textit{gates}, act on one or more qubits and implement unitary transformations. An important example is the \textit{SWAP} gate, which exchanges the states of two qubits and is composed of three simpler two-qubit gates, making it a relatively expensive operation. Gates form the building blocks of larger computational structures.

Analogously to classical programs, a \textit{quantum circuit} specifies an initial state, applies a sequence of gates, and concludes with a measurement. Measuring a qubit collapses its state to a classical outcome, irreversibly eliminating any superposition. The physical realization of qubits and gates depends on the chosen technology. Qubit states are subject to \textit{decoherence}, a process in which the quantum state naturally evolves into a classical state over time, limiting the duration for which computations can be reliably performed.

\myparagraph{Quantum device technologies}
The promise that quantum computers can efficiently solve certain problems intractable for classical computers \cite{shor_1995, grover1996fastquantummechanicalalgorithm} has driven the exploration of various quantum device realizations \cite{Huang2020, Henriet_2020, trapped_bruzewicz_2019}, each with its specific characteristics. Table \ref{tab:technologies} presents an overview of the most promising technologies.

\textbf{(a) Superconducting} devices are the largest group of current quantum computers \cite{Huang2020} and are implemented predominantly with transmon qubits \cite{Roth_2023} fabricated from superconducting materials. While this technology supports fast gate operations (e.g., \cite{Willow2025, Huang2020}), it remains sensitive to environmental noise and typically exhibits limited coherence times (i.e., how long the qubits can maintain their state), which can present challenges for executing longer quantum circuits \cite{Wang_2020}. Since they do not allow for dynamic hardware reconfiguration and therefore support only the connections between neighboring qubits, applying a two-qubit gate between distant qubits requires finding a path connecting them and applying additional gates to bring them next to each other beforehand \cite{maronese2021quantumcompiling, zhu2025quantumcompilerdesignqubit}. 

\textbf{(b) Neutral atom} devices trap rubidium atoms \cite{Henriet_2020} using optical tweezers \cite{radnaev2025universalneutralatomquantumcomputer}. The tweezers allow for flexible circuit layout and mid-circuit movement of the atoms \cite{Bluvstein_2023}, which enables all-to-all connectivity at the cost of longer execution time \cite{radnaev2025universalneutralatomquantumcomputer}. During the movement, an atom loss can occur, which may require a re-run of the computation.

\textbf{(c) Trapped-ion} devices trap charged atoms with electric and magnetic fields \cite{trapped_bruzewicz_2019}. This technology is characterized by a long coherence time of qubits \cite{Wang2021} and slower gate operations with high fidelity \cite{Schäfer2018}. Since the qubits are confined in space and can be precisely controlled and manipulated using lasers, a mid-circuit qubit movement is possible, enabling all-to-all connectivity \cite{Moses_2023}. 

In this work, we consider a set of recently released or planned for release devices, including: Google Willow \cite{Sycamore_2019} and distributed IBM Flamingo \cite{IBM_roadmap}, both superconducting, trapped-ion Quantinuum Apollo \cite{Quantinuum2024Roadmap}, and a neutral atom device from Infleqtion \cite{radnaev2025universalneutralatomquantumcomputer}. They were chosen due to representing the current state-of-the-art, operating using discrete gates and covering vastly different device characteristics.

\myparagraph{Quantum compilation}
Analogously to classical computing, a quantum circuit must first be transformed before it can run on a quantum device \cite{maronese2021quantumcompiling}. Compilation is usually done in multiple stages, including mapping, routing, optimizing, and translating to the target gate set \cite{kaya_2024, amy_gheorghiu_2020, IBM_qiskit_transpiler}. During mapping, the quantum compiler assigns each logical qubit in the circuit to a physical qubit on the device. To make two-qubit gate execution possible and reduce the following overhead, neighbouring logical qubits should be placed on physically adjacent hardware. However, as that is not always possible, this stage is followed by routing, during which the compiler inserts a routing sequence (typically consisting of additional SWAPs) that moves together the quantum states of the distant qubits that must interact. Choosing the shortest, least noisy route is an important optimization problem. Finally, the compiler needs to rewrite every gate in the circuit into the elementary set supported by the target device. Additionally, compilers usually apply optimizations, which aggressively prune the length and the gate count of the circuit. In this work, we focus on the three mandatory stages of the compilation pipeline and their influence on the error correcting circuits: mapping, routing, and gate-set translation.

\myparagraph{Stabilizer simulation}
Evaluating \gls{qec} schemes at scale requires the ability to simulate large quantum circuits, since executing comprehensive benchmarking directly on quantum hardware remains impractical due to hardware limitations and high operational costs. However, classical simulation of quantum circuits using full state-vector representations quickly becomes infeasible as the number of qubits increases, due to the exponential growth of space (\( \mathcal{O}(2^n) \) complex amplitudes for \( n \) qubits) \cite{Westrick_2024}. Fortunately, quantum circuits composed entirely of Clifford operations can be simulated efficiently using stabilizer simulation \cite{chp}. This approach is based on \emph{stabilizer formalism} \cite{Nielsen_Chuang_2010}, in which each quantum state is characterized by its stabilizer group, e.g. a set of mutually commuting Pauli operators \( \mathcal{S}\) such that a pure state \( \ket{\psi} \) is uniquely defined by the condition \( S\ket{\psi} = \ket{\psi} \) for all \( S \in \mathcal{S} \). Stabilizer simulation tracks the stabilizer group rather than the full state vector, allowing it to keep both the time and the space growth polynomial \cite{chp}. This makes it especially suitable for simulating \gls{qec} codes, which predominantly use Clifford operations. In this work, we are using Stim \cite{framework_stim_2021}, which is the current state-of-the-art, to carry out our experiments.

\myparagraph{Quantum noise models}
Quantum devices are inherently noisy and imperfect, which can lead to errors during circuit execution \cite{Preskill_2018}. These errors can degrade measurement fidelity, making them unreliable. To study the impact of such errors without physically running the circuits, various types of noise can be modeled and approximated. To make the noise models compatible with stabilizer simulation, they can be approximated at the circuit level as randomly applied Pauli gates. This technique, which we also use in this work, is called Pauli twirling approximation \cite{twirling_2013}. 

Chatterjee et al. \cite{qpandora_chatterjee_2025} proposed a split of circuit-level noise models into phenomenological and code-capacity models. Phenomenological models represent errors caused by measurement or reset operation. Code-capacity models cover: \circled{1} Depolarizing error: representing loss of quantum information in a qubit due to interaction with the environment. This approximation does not allow for precise representation of amplitude and phase-damping errors, as that would require going outside the Pauli twirling. \circled{2} Gate error: caused by imperfect quantum gate applications. \circled{3} Leakage error: happens when a qubit shifts out of its computational space (for example, to a state like \( \lvert 2 \rangle \), when the computational basis is \( \{ \lvert 0 \rangle, \lvert 1 \rangle \} \)), usually due to applying faulty operations. \circled{4} Crosstalk error: when an operation applied to one qubit unintentionally alters the state or behavior of another qubit. Table \ref{tab:error_rates} presents the probabilities of the presented circuit-level errors across technologies and artificial noise models we use in this work.

\myparagraph{Quantum Error Correction (QEC)}
Quantum states are constrained by the no-cloning theorem \cite{no_cloning_1982}, which, for a long time, made correcting the noise seem impossible. A breakthrough was made by Shor, who proposed a way to overcome that issue \cite{shor_1995}, laying the foundation for the field of \gls{qec}. The \gls{qec} codes, their families, and characteristics are discussed in detail in Section 3. 

\aleksandra{Moved here from taxonomy:}
The majority of \gls{qec} codes can be described by $[[n,k,d]]$, where $n$ is the number of physical qubits used to encode $k$ logical qubits (protected states) and $d$ describes the distance of the code, which is the smallest number of physical qubits that must be corrupted before an error can flip a logical state into another valid logical state, meaning we cannot detect the error anymore \cite{Roffe_2019}. Notably, $n$ is not the full amount of qubits necessary to execute the code, as it does not account for ancilla qubits used for syndrome measurement. A metric presenting the logical qubits to all physical qubits ratio is the net encoding rate: $r = \frac{k}{n+c}$ \cite{Bravyi2024}. Furthermore, the distance correlates to the number of errors the code can fix: $t = \lfloor \frac{d-1}{2} \rfloor$ \cite{Roffe_2019}. Finally, each code has a property called fault-tolerant threshold, which is the maximum physical error rate the code can tolerate. The threshold changes depending on the type and severity of noise applied. 

According to Nielsen et al. \cite{Nielsen_Chuang_2010}, \gls{qec} consists of three steps: \circled{1} \textbf{Encoding}: The protected quantum state is encoded into a quantum error-correcting code by entangling it with multiple physical qubits, which are then collectively entangled with the ancillary qubits prepared in known states.. \circled{2} \textbf{Syndrome Measurement}: Once the code has been affected by noise, the ancilla qubits are measured in a process called syndrome measurement, which detects whether errors have occurred. If errors are found, the measurement outcomes are passed to a classical decoder that identifies and locates the errors to determine the appropriate correction~\cite{decoding_2023}. \circled{3} \textbf{Recovery}: A correction is applied, typically leveraging the fact that Pauli gates are self-inverse, to return the quantum system to its original state.

In this work, we consider two decoding algorithms: \gls{mwpm}~\cite{pymatching_higgott_2025}, based on the graph matching problem, and \gls{bposd}~\cite{bposd_roffe_2020}. They were chosen due to being effective with all the codes we explored and having a well-established, open-source implementations.
