# Supplementary material for: ECCentric: An Empirical Analysis of Quantum Error Correction Codes
Source: arXiv:2511.01062 source file (2026-08-18)
Supplement: Supplementary file 2 [file eccentric_detailed.tex]

\section{The \projectname{} Framework}
%\begin{figure}[htbp]
%    \centering
%    \input{figures/setup_general}
%    \caption{Design of the experimental setup. \aleksandra{There should be input on the left} \pramod{can this figure be made "super detailed" to show different device types, etc.}}
%    \label{fig:setup_general}
%\end{figure}

%\input{tables/scope_coverage_minimal}

In this section, we propose a framework (presented in Fig.~\ref{fig:setup_general}) to evaluate quantum error correction codes in a modular and systematic manner with a focus on their practical application.\\

% How we generally did it
% cases for which we did it and why them
% how we did that in specific cases

\myparagraph{Encoded quantum memory generation}
% How we do it
The pipeline starts with the generation of quantum error-correcting circuits designed to protect one or more logical qubits (encoded quantum memories). Circuit generation supports arbitrary numbers of error-correction cycles and code distances for all codes with a flexible distance parameter. Additionally, \projectname{} enables the generation of codes with the maximal feasible distance tailored to a specific hardware topology, without introducing unnecessary overhead. The generation of these encoded quantum memories leverages established tools and libraries, which we trust to provide circuit constructions that are optimal in terms of gate count and circuit depth and which we further modified to ensure that no noise is introduced during circuit synthesis.

% What we provide
We include the following quantum error-correcting codes, as introduced in Section~\ref{sec:taxonomy}: 

\circled{1} \textbf{Rotated surface code}: Widely regarded as the current state-of-the-art due to its high fault tolerance and practical feasibility \cite{PhysRevLett.129.030501}, this code was generated using the native Stim implementation. The maximal code distance for a given hardware topology supports only odd distances, as the threshold for correctable errors is $\lfloor (d+1)/2 \rfloor$ \cite{Fowler_2012}. Although even distances are theoretically possible, they do not provide significant performance improvements.

\circled{2} \textbf{Gross code}: Introduced as a qubit-efficient alternative to the surface code, this code provides comparable error protection while requiring fewer physical qubits \cite{Bravyi2024}. We generated it using an adapted implementation from \cite{gong2024lowlatencyiterativedecodingqldpc}, which reproduced the results from original work \cite{Bravyi2024} within Stim. The Gross code has a fixed distance of 12.

\circled{3} \textbf{Triangular color code}: Selected due to recent findings that, despite being somewhat more susceptible to noise than the surface code, it may achieve greater qubit efficiency as physical error rates improve \cite{lacroix2024scalinglogiccolorcode}. Additionally, it supports more efficient \gls{ft} gate implementations. We generated this code by adapting an open-source Stim module from \cite{lee2025color}. As with the surface code, only odd distances were considered during finding maximal distance for a given topology in order to avoid unnecessary overhead \cite{Chamberland_2020_triangle}.

\circled{4} \textbf{Concatenated Steane code}: Selected for its potential to outperform the triangular color code in terms of logical error rates \cite{Pato_2024}. Our implementation follows the construction proposed in \cite{Pato_2024} and extends it by adding an additional layer of concatenation, resulting in a novel $[[343,1,27]]$ code. The design prioritizes optimal circuit depth and size. The only available code distances are 3, 9, and 27.

\circled{5} \textbf{Bacon-Shor code}: Chosen due to being particularly suited to realistic noise models of trapped-ion devices \cite{ion_traps_2020}. We employed an implementation based on a square lattice layout, which maximizes code distance, following \cite{gidney2023baconthreshold}. Due to majority voting step of Bacon-Shor code, its distance needs to be odd \cite{Brooks_2013}.

\circled{6} \textbf{Heavy-hex code}: Specifically designed for heavy-hex lattice architectures, this code offers error protection comparable to that of the surface code while requiring a sparser qubit connectivity graph \cite{Chamberland_2020}. We adapted the code generation from publicly available educational materials \cite{heavyhexdemo}. As with the surface code, only odd distances were generated to avoid introducing unnecessary overhead \cite{Chamberland_2020}.

All the codes are initially generated in the Stim format \cite{framework_stim_2021} and then translated into Qiskit \cite{javadiabhari2024quantumcomputingqiskit} format to allow for transpilation—i.e., translation, mapping, and routing on target hardware. This translation step is essential to realistically reflect the behavior of physical systems. We used the qiskit-qec library \cite{qiskitqec} tool for circuit translation, which replaces Stim-specific operations with equivalent Qiskit-native gate sequences. For instance, the MRX gate is translated into the sequence H-M-R-H, preserving circuit semantics. The correctness of translation was verified manually and automatically on code samples.
\\

\myparagraph{Translation}
% How we do it
Before execution, the generated circuit must be transpiled to match the gate set supported by the target device. For full simulation in our pipeline, the circuit must conform to the gate set available both in Qiskit and in Stim.
%, which includes the following operations: {X, Y, Z, CX, CZ, CY, H, S, S\_dag, SWAP, RESET, MEASURE, BARRIER}. 
For this task \projectname{} supports both Qiskit \cite{javadiabhari2024quantumcomputingqiskit} and TKET \cite{Sivarajah_2020_tket} translators, selected due to their translation performance and effectiveness \cite{benchpress_2025}. Only the translation functionalities of these SDKs are utilized. We initially evaluated BQSKit \cite{doecode_58510_bqskit} as well, but found that it removed operations deemed redundant based on known input states—behavior that interferes with error detection. As a result, BQSKit was excluded from our experiments.

The pipeline currently includes gate set definitions for Qiskit/Stim, IBM Heron, and Quantinuum H2, chosen for their accessibility, real-world relevance, and diversity of gate types. Although we provide those alternatives for partial experiments, full execution requires adherence to the Qiskit/Stim gate set. To ensure this compatibility, an additional translation step is performed during the mapping and routing stage, with all compiler optimizations disabled. This guarantees that any non-supported gates are correctly converted using Qiskit’s translation tools. The mapping and routing process may introduce additional SWAP gates, but since these are natively supported by Stim, therefore no further decomposition is required.
\\

\myparagraph{Mapping and routing}
% How we do it
Before execution, a quantum circuit must be mapped onto the device topology, followed by routing to ensure that all two-qubit gates can be physically implemented. In \projectname{}, this stage is carried out by the Qiskit Transpiler \cite{IBM_qiskit_transpiler}. In addition, we implement a Qubit Tracker mechanism that tracks the mappings between physical and logical qubits throughout the circuit. This is particularly important when SWAP gates are introduced, as the noise model must reference the correct physical qubit. Our qubit tracking system respects the ordering of SWAP operations and concurrently executed gates as defined by Stim. In future work, this could be extended to support more flexible gate reordering.

% What we provide
Our setup supports all Qiskit transpilation parameters. Specifically, we include three initial layout strategies ("Trivial", "Dense", and "Sabre") and three routing algorithms ("Basic", "Stochastic", and "Sabre"). We also support the Lookahead mapping algorithm, but excluded it from our experiments due to its prohibitively long execution times on larger circuits and topologies.
\\

\myparagraph{Backends}
% How we do it
All backends used in this work were artificially created based on BackendV2 from Qiskit \cite{javadiabhari2024quantumcomputingqiskit}. Each custom backend is characterized by its topology (coupling map), represented as a graph of qubit connections, and, where applicable, by qubit-specific properties such as T1 and T2 times.

% what we provide
\projectname{} supports generation of custom artificial topologies: line, heavy-hex, grid, cube and fully connected topology of a specified number of qubits. For simplicity, the grid topology is always a square, and the cuboid is always modeled as a cube. When the requested number of qubits is not a perfect square or cube, we take the floor of the value to construct the topology.

In addition to synthetic topologies, the pipeline incorporates backends modeled after real devices: Google Willow \cite{Willow2025}, Quantinuum Apollo \cite{Quantinuum2024Roadmap}, Infleqtion \cite{radnaev2025universalneutralatomquantumcomputer}, and IBM Flamingo \cite{IBM_roadmap}. These devices were selected due to their current or projected status as state-of-the-art platforms in terms of error rates. Since Google Willow and Infleqtion currently support a limited number of qubits, and since our focus is on evaluating code performance for future architectures, we scale these systems up in simulation—Google Willow by a factor of 3 (to 315 qubits) and Infleqtion by a factor of 16 (to 384 qubits). In contrast, although Quantinuum Apollo is expected to support thousands of qubits, we downscale it to 768 qubits for simulation feasibility, which still enables meaningful evaluation of large-scale codes. 

In the original Infleqtion device paper \cite{radnaev2025universalneutralatomquantumcomputer}, shuttling was not used to improve the general error rates. Since it is an important quality of neutral atom device, our simulation provides two versions of the Infleqtion backend: with shuttling enabled and disabled. To simulate shuttling, we start with a grid topology and then add connections to achieve full connectivity, while marking which qubit pairs were connected via those additional links. These remote connections are assigned distinct durations and error rates. Since tracking a dynamically changing coupling map during shuttling would significantly slow down simulations and complicate noise modeling, we simplified the shuttling process by assuming that for every remote two-qubit gate, one qubit is physically moved adjacent to the other, the gate is performed, and then the qubit returns to its original position. The shuttling error for Infleqtion is modeled as decoherence proportional to the shuttling time, which is calculated based on the Euclidean distance between qubits multiplied by the distance between neighboring qubits, divided by the maximum shuttling speed that introduces no error, as proposed in \cite{Bluvstein_2022}. 

Quantinuum Apollo, as a trapped-ion device, also supports shuttling, with shuttling errors derived directly from the characteristics of the Quantinuum H2 system \cite{Quantinuum2024Roadmap}. These devices achieve all-to-all qubit connectivity through a combination of fully connected zones and shuttling between them. In our model, we simplify this topology by treating all non-neighboring qubit interactions as requiring shuttling. This decision was motivated by the lack of detailed information regarding the planned number and configuration of zones in Quantinuum Apollo and its predecessor, Quantinuum Sol \cite{Quantinuum2024Roadmap}, as well as the significantly different topology of Quantinuum H2, which makes accurate extrapolation challenging \cite{Quantinuum2024Roadmap}.
\\

\myparagraph{Representation change}
% How we do it
To enable effective simulation of the circuit, it is then translated to Stim to utilize its support for stabilizer formalism. Such a prepared Stim-circuit adheres to the supported gate set and contains additional SWAP gates. The translation is done using qiskit-qec.
\\

\myparagraph{Adding noise}
% How do we do it
Noise addition is done after translation, to ensure adherence to stabilizer simulation constraints and to fully utilize the available granularity of the noise specification. It is applied by iterating through the Stim circuit and inserting gate-level noise according to a provided configuration. This model supports pre-, mid-, and post-gate error insertion based on the gate type, its duration, and device-specific parameters. The injected noise includes: \circled{1} Depolarizing errors on single- and two-qubit gates \circled{2} Idle noise modeled as single-qubit depolarization on inactive qubits \circled{3} Leakage errors applied as a Pauli error with probability 1.0 and optionally propagated to the gate partner \circled{4} Crosstalk modeled as unintended errors on nearby qubits during multi-qubit operations \circled{5} Correlated parity measurement errors, although due to the translation which the circuits are undergoing, no such operations are included in our circuits. Our approach generalizes the noise model injection mechanism introduced in \cite{comparison_honeycomb_vs_surface_2021}, extending it to support dynamic qubit tracking, leakage and crosstalk errors, realistic gate durations, and backend-specific characteristics.

% What we provide
We currently provide several standard error models, including SD6, EM3, and SI1000, based on \cite{comparison_honeycomb_vs_surface_2021}. Their error characteristic is presented in Tab.~\ref{tab:error_rates}. We modified the SI1000 model to apply noise to all two-qubit gates, not just CZ gates. While the original model reflects superconducting hardware assumptions (favoring a CZ-based gate set), our compilation pipeline retains Qiskit/Stim’s gate set. Thus, for consistency, we extend the noise model to uniformly treat all two-qubit operations.

We also support realistic, device-specific noise models tailored to the topologies of selected hardware platforms: Infleqtion, Google Willow, IBM Flamingo, and Quantinuum Apollo, with error rates specified in Tab.~\ref{tab:error_rates}. Remote connections—present in IBM Flamingo and used to emulate qubit shuttling in Infleqtion and Apollo—are identified by analyzing the physical qubit locations tracked by the Qubit Tracker. If a two-qubit gate is detected to span a remote connection, its execution time is increased, and in the case of IBM Flamingo, a higher error probability is applied accordingly. For Google Willow and Quantinuum Apollo, due to how their noise characterizations are provided, we directly apply constant idle errors. For Infleqtion and IBM Flamingo, idle noise is derived from reported $T_1$ and $T_2$ coherence times of specific qubits in combination with actual gate durations. Amplitude damping and phase decay are then approximated using Pauli twirling \cite{twirling_2013}, following the methodology described by Tomita et al. \cite{surface_vs_realistic_noise_2014}. This technique enables decoherence processes to be expressed as equivalent Pauli noise channels, ensuring compatibility with efficient stabilizer-based simulation.
\\

\myparagraph{Decoding}
% How we do it:
Initially, the framework compiles the circuit into a detector error model (DEM) \cite{derks2024designingfaulttolerantcircuitsusing}, which describes how physical errors propagate through the circuit, trigger detection events (syndromes), and may flip logical observables, resulting in corruption of the encoded information. This model is then used to simulate error data, mimicking how errors would appear during execution. Based on this data, the decoder attempts to infer the most likely underlying error pattern. It then checks whether applying this correction would have prevented the corruption. By repeating this process many times, we estimate the logical error rate, defined as the fraction of runs where the decoder fails to correct the error.

% What we provide
The framework is equipped with established decoding tools which support the stabilizer simulation and Stim execution: BP+OSD and MWPM. Our choice was motivated using the most general ones, working across all the codes. There are many upcoming decoders, often code-specific, which are able to generate better results \cite{Kubica_2015, Kubica_2019, gidney2023newcircuitsopensourceChromobius}, but we decided on adhering to generality to avoid the problem of choosing the state-of-the-art codes for each code and time constraints, which are out of scope of this work. Experimental comparisons indicate that the performance of the selected decoders is comparable to that of specialized decoders for realistic noise model, making them sufficiently representative. Additional details are provided in the appendix.

\begin{figure}[t]
    \centering
    \includegraphics[scale=0.35]{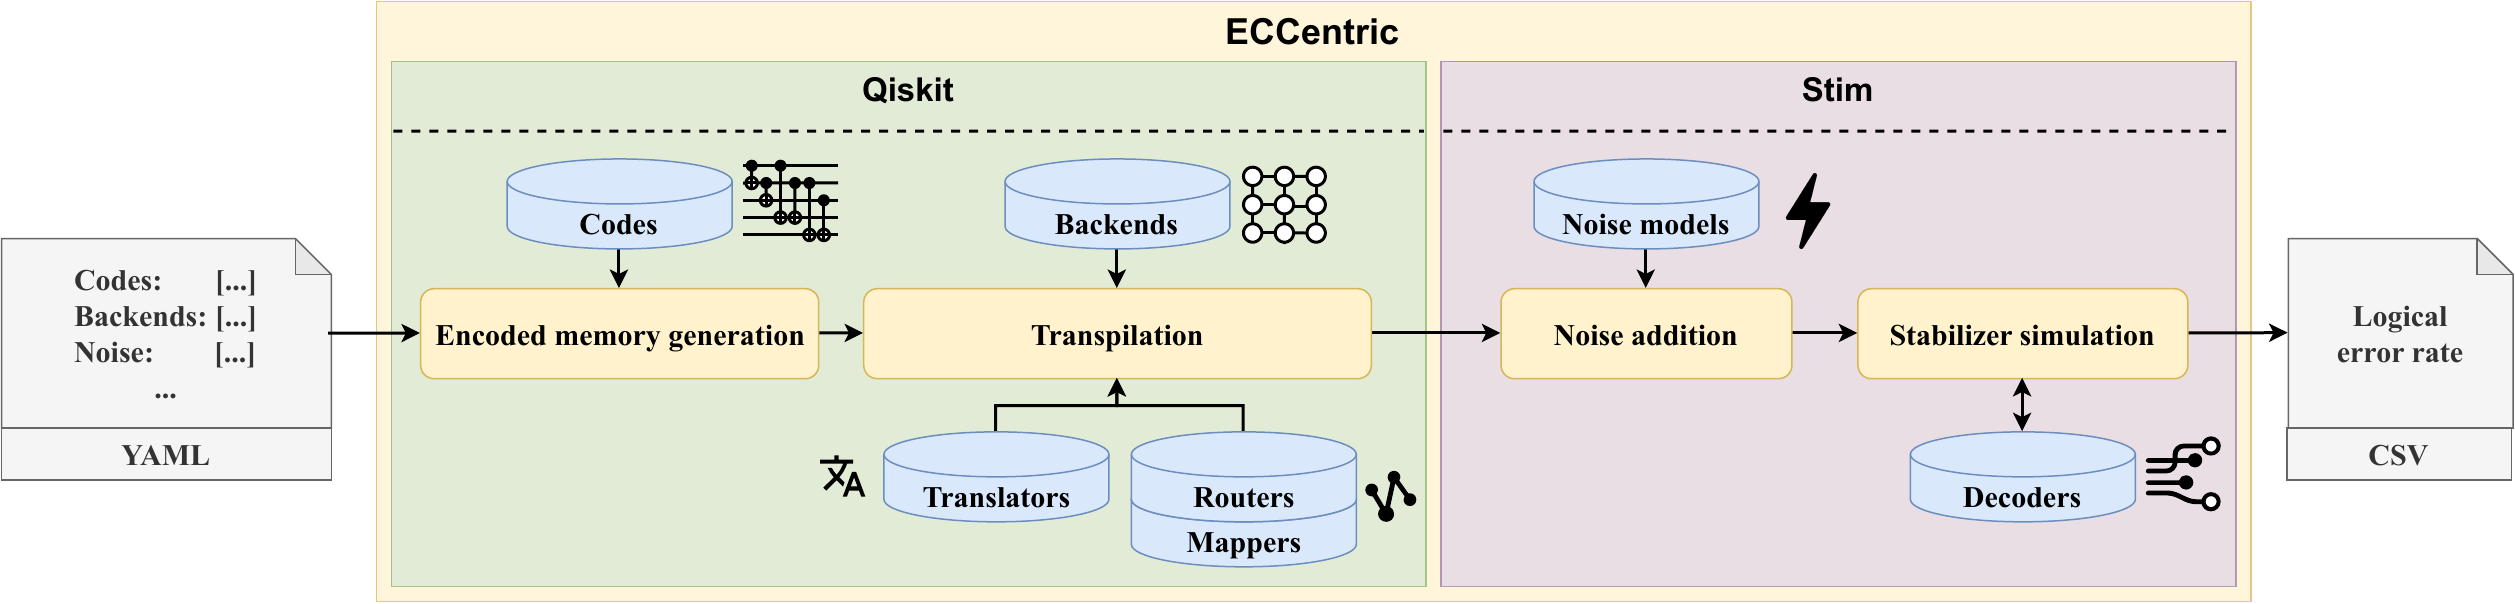}
    \caption{Design of the experimental setup. \pramod{I find the figure a bit boring, TBH. I was wondering if we could make it a bit interesting, e.g., using some icons, figures, etc. We need to discuss it in person with Jannik and Manos.} \pramod{is it the architecture of the eccentric framework? if so, then spell this out. Also describe/state that the architecture is designed to completely modular/extensible to systematically study different aspects of the work. Also, it would be good mark respective subsections in the figure.}}
    \label{fig:setup_general}
\end{figure}

\subsection{Experiments design}
For all experiments, the codes were generated using their maximal distance possible on a chosen topology, with the number of cycles set equal to the code distance. This approach showed better results compared to using a fixed number of cycles \cite{Fowler_2012, Dennis_2002}. \aleksandra{Mention basis} \aleksandra{would be nice to show that in the appendix if there's time to spare}

In experiments that do not explore specific configurations for translation, mapping, and routing, we use Qiskit transpilation with the default settings and optimization level set to 0. This results in Qiskit's basic translation to the gate set supported by Qiskit/Stim \cite{framework_stim_2021}, "Trivial" mapping, and "Sabre"-based routing \cite{IBM_qiskit_transpiler}. We avoid applying additional optimizations because we aim for a possibly consistent baseline for all codes.

For the majority of experiments that do not require a specific noise model, we use the SI1000 noise model with an error probability of 0.004. This error type and value were chosen experimentally as severe enough to highlight differences in code effectiveness while still preserving their error-correcting capabilities. Detailed results can be found in the appendix \aleksandra{TODO: add to appendix}.

All experiments employed the BP+OSD decoder. For the Bacon-Shor and Steane codes, we used parity-check matrix decoding, while batch decoding was applied for all other codes. These choices were made based on experimental evaluation, as they yielded the best logical error rates under the realistic artificial noise model SI1000. The corresponding results are included in the appendix. For all experiments using a realistic noise model, the approximate\_disjoint\_errors setting in Stim is enabled during compilation of the detector error model to approximate the correlated error processes as independent. Otherwise, the complexity of noise makes the decoder ineffective.

Data for each experiment was collected over 1000 executions. For hardware-related experiments, the pipeline execution was repeated, starting from the translation stage to account for variability in mapping and routing, thereby capturing the effectiveness of codes across varying topologies. Each run consisted of a single shot.
