# Supplementary material for: ECCentric: An Empirical Analysis of Quantum Error Correction Codes
Source: arXiv:2511.01062 source file (2026-08-18)
Supplement: Supplementary file 3 [file full_related_work.tex]

\section{Related Work}
% one sentence to introduce each bucket
% then name works
% then unfortunately what's wrong with them
\myparagraph{Benchmarking in quantum computing}
As the field of quantum computing grows, the recent comprehensive surveys by Lorenz et al. \cite{benchmarking_lorenz_2025} and Proctor et al. \cite{benchmarking_survey_proctor_2024} underlined the importance and listed the ongoing benchmarking efforts to guide future hardware and software development across the entire software stacks. There are already well-established benchmarking suites like QASMBench \cite{benchmark_qasmbench_2022}, MQT Bench \cite{Quetschlich_2023}, and SupermarQ \cite{ benchmark_supermarq_2022}, allowing for the assessment of quantum software performance. There are efforts focused on the evaluation of quantum software development kits \cite{benchpress_2025} and finally, the benchmarking capturing the performance of qubits \cite{ibm_layer_fidelity_2023}. However, all the benchmarking studies referenced above are \gls{qec}-agnostic and hence orthogonal to this work.

Although many comprehensive benchmarking efforts are emerging, systematic and wide-ranging benchmarking of \gls{qec} codes remains scarce. Several studies have explored specific \gls{qec}-related issues -- for example, Kurman et al. assessed the impact of low-latency feed-forward operations in fault-tolerant quantum computing \cite{bechmarking_controller_kurman_2024}, while Zhao et al. benchmarked the effectiveness of \gls{ml} techniques in capturing long-range dependencies to enhance decoding performance \cite{benchmarking_ml_qec_zhao_2024}. Other notable benchmarking efforts were done by Finsterhoelzl et al., who compared the effectiveness of repetition codes transpiled to a superconducting quantum processor and a Nitrogen-vacancy center quantum register in simulation and experiment \cite{small_codes_on_hardware_2022}, and by Huang et al., who compared the effectiveness of Shor and Steane syndrome extraction methods on a Bacon-Shor code on a trapped ions device \cite{comparison_shor_vs_steane_on_beacon_trappedion_2024}. While these works highlight progress in simulating noise models and practical implementations, they often focus on simplistic codes (e.g., the repetition code) or specific components of the \gls{qec} technique. Broader comparative studies have primarily evaluated multiple quantum error correcting codes under idealized, uniform error models to estimate fault-tolerance thresholds \cite{comparison_11codes_2009, comparison_many_codes_huang_2019}. In contrast, this work assesses the performance of various \gls{qec} codes under realistic, device-tailored noise models and practical constraints, aiming to evaluate their applicability on mid-term quantum devices.

\myparagraph{Benchmarking frameworks}
Despite limited benchmarking works in the field of \gls{qec}, there are multiple ongoing efforts aiming to create a framework allowing for simulation and testing of code effectiveness. The most popular tool is Stim \cite{framework_stim_2021}, allowing for experimenting with codes using flexible noise models and simulating the results using stabilizer simulation. However, since Stim is limited to stabilizers, it is not suitable for end-to-end simulation of deploying \gls{qec} codes on devices using a quantum software stack and how it can influence their effectiveness. Similarly, Grurl et al. proposed a framework automating the process of applying error correction and allowing noise-aware simulation of the protected circuits \cite{framework_wille_2023}. However, the framework is also under development and still limited in the codes and error models it supports (i.e., currently it does not support subsystem codes or specific gate-level noise injection). A more noise-focused framework was presented in 2020, when IBM extended the Qiskit-Ignis library to provide tools for quantum hardware verification and noise characterization, by a module introducing topological codes in order to evaluate the performance of current quantum computing devices, particularly concerning their ability to support quantum error correction techniques \cite{framework_wootton_2020}. Unfortunately, the library is currently deprecated. Finally, there are also works limited only to a specific family of codes, such as Kang et al., which allows for a simulation of \gls{qldpc} codes \cite{framework_kang_2025} and Mitsuki et al., which provides an exploration of numerical simulation for rotated surface code \cite{framework_mitsuki_2024}. Our work aims to provide a framework allowing for the evaluation of a wide spectrum of codes, using precise noise models and including the software stack influence, without resigning from efficient simulation.

\myparagraph{Code design}
General \gls{qec} codes, not designed for a particular device, may provide suboptimal results on real architectures. There are ongoing efforts to maximize the effectiveness of the existing \gls{qec} codes and methods by modifying them and adjusting for the specific use-cases. Guo et al. proposed a simplistic \gls{qec} code designed specifically for a distinct type of noise on three distinct quantum computing platforms \cite{new_code_guo_2021}, whereas Stein et al. proposed a method for integrating hybrid \gls{qec} codes with the constraints imposed by a specific architecture, demonstrating its effectiveness by showing how the combination of the surface code and the gross code helps manage the trade-offs inherent to each \cite{hetec_2025}. Although in this work we do consider a code created specifically for the target device topology (heavy-hex code), the problem of code design is out of the scope of our project.

\myparagraph{Theoretical comparisons}
The majority of \gls{qec} code evaluations rely on direct comparisons between two codes, typically either through theoretical predictions, as did Steane et al. in 2003, comparing the theoretical qualities of Golay and Hamming codes \cite{golay_vs_hamming_2003}, or by tests under phenomenological or uniform noise models. Currently, the effectiveness of different codes, often during their introduction, is juxtaposed with the effectiveness of surface codes, as in the case of Steane code \cite{steane_vs_surface_2017}, honeycomb code \cite{comparison_honeycomb_vs_surface_2021}, BB \gls{ldpc} codes \cite{Bravyi2024}, and color codes \cite{surface_vs_color_2007, comparison_surface_vs_color_2024}. Unfortunately, theoretical comparisons are not enough, since the idealized error models usually underestimate the severity of noise encountered in real devices, rendering claims of effectiveness overly optimistic. In this work, we evaluate the codes using both idealized error models and more realistic alternatives for accurate usability assessment.

% Not going well with the flow and not very important showing how limited conectivity influences qldpc codes but mathematically on a graphs \cite{qldpc_connectivity_2022}

\myparagraph{Practical comparisons}
The need to analyse the applicability of the \gls{qec} code in real-life use cases motivates the code comparisons with a more practical angle. An example of such works could be a comparison of predicted resource overheads of the codes \cite{resource_estimation_suchara_2013, steane_reed_vs_surface_2017} or the effectiveness of codes with different decoders as presented in \cite{surface_xzzx_vs_decoders_2023}. Practical comparisons often also accompany works on \gls{qec} compilers, especially those focused on securing the correcting capabilities of the codes, such as \cite{qecc_synth_2025}, in which the effectiveness of the proposed mapper with various codes was explored.

The most common approach to exploring the suitability of the codes on real devices is simulating their effectiveness against realistic noise models. For example, Benito et al. compared the effectiveness of the surface code, Floquet honeycomb code, and heavy-hex code on a heavy-hexagonal topology under such noise conditions \cite{heavyhex_2025}. Similarly, Debroy et al. evaluated the rotated surface code, Bacon-Shor code, and two variants of the Shor code against realistic trapped-ion noise \cite{bacon_surface_shor_trapped_ion_2020}. Additional studies include work by Tomita et al. and Chatterjee et al., who tested surface codes against realistic noise \cite{surface_vs_realistic_noise_2014, qpandora_chatterjee_2025}; Gutiérrez et al., who examined the Steane code \cite{steane_noise_comparison_2015}; and Fan et al., who investigated hypergraph \gls{qldpc} codes \cite{comparison_hypergraph_qldpc_2020}. Finally, Iyer et al. proposed a diagnostic method for estimating the efficiency of concatenated codes under noise observed on real quantum devices \cite{estimated_concantanated_2022}.

Unfortunately, these works focus on a limited subset of tools or codes. Our work adopts a similarly practical perspective while providing a systematic evaluation of a broader range of codes under realistic noise models, taking into account resource overheads as well as the impact of decoders and compilation stages.
% TBH 

\myparagraph{Surveys}
With new \gls{qec} codes fastly emerging, there also emerges a need to arrange, summarize, and survey the existing codes. There are existing works trying to bring closer the theoretical characteristics and mathematical backgrounds of codes, such as \cite{survey_matsumoto_2021, survey_noise_adapted_2022, theoretical_overview_2023}, and works aimed at a more general audience \cite{qec_for_dummies_2023, magic_mirror_2024}. However, the majority focuses on presenting the chronological development of the codes and not on the codes' overlapping characteristics, which was the main goal of our project. 

Additionally, although not a survey, a very important source of knowledge regarding error correction codes is Error Correction Zoo \cite{ErrorCorrectionZoo}, a collaborative effort to catalog existing codes, their properties, and associated error rates. However, due to its community-driven nature, the information is often presented in a non-uniform format, which can hinder direct comparisons between codes.

\textbf{How our paper differs?}
Compared to the existing works, this paper presents a systematic benchmarking of multiple \gls{qec} codes with a focus on their practical application, tested against real devices, compilers, and noise models. Our framework is equipped with multiple \gls{qec} codes, architectures, compilers, noise models, and decoders, and it can be easily further extended to adjust to the growing field. Our survey was aimed at a broad audience with a focus on code taxonomy, therefore their characteristics, overlaps, and differences, to better present the code's qualities and constraints.
