# Supplementary material for: ECCentric: An Empirical Analysis of Quantum Error Correction Codes
Source: arXiv:2511.01062 source file (2026-08-18)
Supplement: Supplementary file 4 [file taxonomy_ext.tex]

\section{Quantum Error Correction Codes Taxonomy}
% Put that not as background ++ but move it to after the research scope as contribution
% Make it more active
\label{sec:extended_taxonomy}
\gls{qec} can be achieved utilizing a myriad of different mathematical properties, giving rise to an enormous variety of codes with distinct characteristics, requirements, and error-correcting capabilities. To bring structure to this diversity and to enable systematic evaluation, we introduce a strict taxonomy that groups codes into families based on shared principles and traces their derivatives. We characterize five families: stabilizer, subsystem stabilizer, \gls{qldpc}, concatenated, and topological codes, emphasizing both their similarities and their differences. Tab.~\ref{tab:code_categories} provides an overview of the code classifications, while Tab.~\ref{tab:code_stats} compares the overheads of typical representatives from each family. The corresponding code structures are illustrated in Fig.~\ref{fig:all_codes}.

% This paper describes stabilizers and qldpc but is not very good:
% https://www.jstage.jst.go.jp/article/transfun/E104.A/12/E104.A_2021EAI0001/_pdf/-char/en

% CODE
% THIS GROUP IS BASED ON X (THEORETICAL CONCEPT) WHICH IS USED IN THIS WAY
% HOW THEY ARE SIMILAR/DIFFERENT FROM PREVIOUS
% REQUIREMENTS
% PARAMETERS AND CAPABILITIES
% CODE EXAMPLE AND ITS MAIN CHARACTERISTIC

\subsection{Stabilizer Codes}
Stabilizer codes utilize the concept of stabilizer formalism \cite{gottesman1997stabilizercodesquantumerror}. They are defined by a group of mutually commuting Pauli operators \( \mathcal{S}\) such that a pure state \( \ket{\psi} \) is uniquely defined by the condition \( S\ket{\psi} = \ket{\psi} \) for all \( S \in \mathcal{S} \). Those operators are used to entangle data qubit with ancilla qubits prepared in knows states, which are then measured in a procedure called syndrome measurement extraction. Since they anti-commute with all the other Pauli operators, they allow to detect errors \cite{Roffe_2019}.

For example, consider the stabilizer \( S = X_1 X_2 X_3 X_4 \), which acts on four data qubits (is of weight-four). To measure this stabilizer, an ancilla qubit is first prepared in the \( \ket{+} \) state. Then, CNOT gates are applied with each data qubit (qubits 1 through 4) as the \textit{control} and the ancilla as the \textit{target}. Finally, the ancilla is measured in the \( X \)-basis. If no error has occurred or if occurring error commutes with the stabilizer (i.e. error X), the stabilizer measurement yields \( +1 \). If a \( Z \) error occurs on any of the data qubits, it anti-commutes with the corresponding \( X \) in the stabilizer, flipping the stabilizer’s sign to \( -1 \), and the measurement outcome shows that an error has occurred. 

The compatibility of stabilizer codes with efficient classical simulation techniques has made them the foundation for most quantum error correction schemes studied to date. All code families discussed in this work are based on the stabilizer formalism.

\subsection{Subsystem Stabilizer Codes}
The family of subsystem codes protects logical information by encoding it into a subsystem of the Hilbert space, rather than a subspace \cite{aly2006subsystemcodes}, generalizing the approach of first error correction codes \cite{shor_1995}. This introduces additional degrees of freedom, called gauge qubits, whose states do not influence the logical information. In a classical sense, we can see them as non-important bits (e.g., 11X). Because of this generality, the family of subsystem codes the broadest of \gls{qec} codes families, containing almost all the known codes.

In practical applications, focus is placed on the subclass of stabilizer subsystem codes, which utilize the stabilizer formalism for efficient simulation and leverage a non-trivial gauge group to reduce the complexity of syndrome extraction by replacing some stabilizers with lower-weight gauge operators \cite{Higgott_2021} -- to distinguish this subclass, we refer to it as subsystem stabilizer.

\myparagraph{Bacon-Shor code}  
A well-known example of a subsystem stabilizer code is the Bacon-Shor code \cite{Bacon_2006}. The code is defined on a rectangular lattice of size \(m_1 \times m_2\), with parameters \([[m_1 m_2, 1, \min(m_1, m_2)]]\) \cite{egan2021faulttolerantoperationquantumerrorcorrection}. Local \(XX\) and \(ZZ\) measurements between neighboring qubits (gauge operators) introduce gauge degrees of freedom, while the stabilizers are formed by products of these operators along entire columns and rows, respectively, as shown in Fig.~\ref{fig:bacon_shor}. Asymmetry in the lattice dimensions can bias the code toward stronger protection against either \(X\)- or \(Z\)-type errors, at the cost of reduced code distance. A symmetric lattice maximizes the code distance but may be less flexible for certain hardware layouts.

%The net encoding rate of the code is then $\frac{1}{d^2}$, where $d$ is the code distance and $d = m_1 = m_2$.
%which is a subsystem variant of the 9-qubit Shor code \cite{Shor_9Qubit}. 
%If we use the same system size then Bacon-Shor code only needs 4 weight 6 stabilizer instead of the 8 stabilizers which are needed in the nine-qubit shor code (2 weight-6, 6 weight-2 stabilizers). 

\subsection{Topological Codes}
The family of topological quantum error correction codes was first introduced by Kitaev through the toric code \cite{Kitaev_2003}. These codes store quantum information in global, topological features of a qubit lattice, which makes them inherently robust against local errors \cite{bombin2013introductiontopologicalquantumcodes}. The code distance increases with the size of the lattice, enabling stronger protection as the system scales. Topological codes require only local interactions, such as nearest-neighbor connectivity, making them well-suited for implementation on current quantum hardware and, therefore, one of the most widely studied approaches in quantum error correction. In this work, we focus on two representative members of this family:

\myparagraph{Surface code} The most studied member of the family is surface code \cite{Fowler_2012}, widely considered current state-of-the-art in error correction \cite{PhysRevLett.129.030501}. The code is defined on a 2D square lattice where each data qubit typically connects to four others. Weight-four stabilizers act on these nearest-neighbor qubits, with each stabilizer being either \(X\)- or \(Z\)-type, as shown in Fig.~\ref{fig:surface}, where different colors indicating each type. To improve qubit efficiency, the rotated surface code, a variation that preserves the stabilizer structure but swaps the roles of data and ancilla qubits, is often employed. 
%It provides a net encoding rate of $\frac{1}{(2d)^2}$, where $d$ is the code distance.

\myparagraph{Color code} Another promising member of the family is color code \cite{Bombin_2006}. This code is defined on a lattice where each plaquette (a face of the tiling bounded by adjacent qubits) has been assigned a color, but no two neighboring plaquettes can share the same color. The colors correspond to subsets of stabilizers, with each plaquette supporting stabilizers of both an X-type and a Z-type. A prominent member of this family is the \textbf{triangular color code}, defined on a 2D hexagonal lattice (specifically, a 6.6.6 tiling). It is valued for its relatively strong error-suppressing abilities and its major advantage — a set of fault-tolerant gates which can be applied with low overhead, making it an excellent candidate for fault-tolerant quantum computing \cite{bombin2013introductiontopologicalquantumcodes, lacroix2024scalinglogiccolorcode}. Its stabilizers have weight six and act on three-colorable plaquettes, with each qubit connected to three neighbors.
%The code encodes one logical qubit, and its net encoding rate is approximately $\frac{4}{(3d - 1)^2}$.

%
\subsection{Quantum Low-Density Parity-Check Codes}
Quantum Low-Density Parity-Check (QLDPC) codes are a class of stabilizer codes characterized by sparse parity-check matrices, which means that each stabilizer involves only a small subset of qubits~\cite{PRXQuantum.2.040101}. While this sparsity reduces measurement complexity, the codes often require higher or even long-range connectivity between qubits, which poses significant hardware challenges. Despite these demands, a major advantage of certain QLDPC is their efficient scaling: they can maintain a constant ratio of logical to physical qubits (\( k/n \)) while achieving a minimum distance that grows proportionally with the number of physical qubits (\( d \propto n \)), allowing them to protect more logical qubits without increasing the overhead per logical qubit as the system grows.

\myparagraph{Bivariate Bicycle (BB) codes} \cite{Bravyi2024} are a specialized subclass of \gls{qldpc} codes constructed using matrices derived from certain bivariate polynomials, characterized by regular, repeating stabilizer patterns. This structured design simplifies implementation and enables higher encoding rates and favorable error thresholds. There are many variations of the BB codes \cite{wang2024coprimebivariatebicyclecodes}, with the most prominent being the \textbf{gross code}. The gross code $[[144,12,12]]$, which encodes 12 logical qubits rather than just 1, has gained recent attention for its low net encoding rate \( k/n = \frac{1}{24} \) \cite{Bravyi2024} and its promising performance: using 288 physical qubits, it achieves error correction comparable to the surface code with over 3000 physical qubits. All stabilizers in the gross code have weight six, reflecting the code’s structure where each node connects to six others—four nearest neighbors and two long-range interactions—as illustrated in Fig.~\ref{fig:gross}.

%BB codes are constructed using two distinct cyclic shift matricies A and B. The matricies are based on bivariate polynomials (e.g. $A = x^3 + y + y^2$). Given these two matricies we can define the check matricies of the code by concatenating A and B:\[H_X = [A | B] \quad H_Z = [B^T | A^T] \]
%BB codes are constructed using weight-6 stabilizer on a degree-6 Tanner graph that decompose int two stacked planar fields. 
%Using a depth-7 syndrome measurement cycle and a threshold close to 1\% the authors managed to encode more logical qubits than surface code. 

\subsection{Concatenated Codes}
% CODE
% THIS GROUP IS BASED ON X (THEORETICAL CONCEPT) WHICH IS USED IN THIS WAY
Concatenated quantum error-correcting codes \cite{knill1996concatenatedquantumcodes} encode quantum information by nesting one code within another. Specifically, an outer code encodes the logical qubits, and each physical qubit of this code is further encoded using an inner code. This layered structure allows flexible combinations of codes to improve error correction. 
%A well-known example is the 9-qubit Shor code \( [[9,1,3]] \) \cite{Shor_9Qubit}.
%\myparagraph{Steane Code} \aleksandra{Let's just have concatenated Steane code, we may just mention in the passing that the [7, 1, 3] is also color code but it doesn't matter}
%The $[[7,1,3]]$ Steane code \cite{Steane_96} is the smallest CSS code to correct a single-qubit error. It encodes one logical qubit in seven physical qubits and can correct both X and Z errors. The data qubits for this code can be placed on a plane and each qubit has up to 3 connection points. With that the Steane code is the smallest error correction code. The generators for the $[[7,1,3]]$ code are:

%\[
%\begin{aligned}
%g_{1}^{x} &: \; X\; I\; I\; X\; I\; X\; X, 
%&\qquad g_{1}^{z} &: \; Z\; I\; I\; Z\; I\; Z\; Z,
%g_{2}^{x} &: \; I\; X\; I\; X\; X\; I\; X, 
%&\qquad g_{2}^{z} &: \; I\; Z\; I\; Z\; Z\; I\; Z,
%g_{3}^{x} &: \; I\; I\; X\; I\; X\; X\; X, 
%&\qquad g_{3}^{z} &: \; I\; I\; Z\; I\; Z\; Z\; Z.
%\end{aligned}
%\]

\myparagraph{Concatenated Steane code}
A notable example of a concatenated code is the concatenated Steane code \cite{Pato_2024}, denoted as $[[7^m,1,3^m]]$. It is constructed by recursively concatenating the standard Steane code $[[7,1,3]]$ \cite{Steane_1996} with itself $m-1$ times. This construction allows it to outperform certain color codes, including the triangular color code \cite{Pato_2024}. However, a common drawback of concatenated codes is that their encoding rate decreases exponentially with the concatenation level. Specifically, for the concatenated Steane code, the net encoding rate is given by $r_m = \frac{1}{2 \cdot 7^m}$, indicating that a large number of physical qubits are required to encode a single logical qubit. Furthermore, increasing the concatenation level $m$ introduces larger stabilizers, which increases the syndrome measurement complexity.

%What characterizes them.
%A lot of attention is currently put towards topological codes, especially color codes which gave rise to Floquet Codes and 3D color codes. They are very new, difficult to find, not typical representants and not ready for using so that's why we did not include them here. 
%\jannik{Cited Bombin instead of Kubica because first proposed Color Code was by him, we can add Kubica as well}

%\input{tables/quantum_error_codes_comparison}

\subsection{Architecture-specific Codes} % honorary mentions
Additionally, a different approach to \gls{qec} has been explored in which codes are designed specifically to match the constraints of particular quantum hardware. While such codes may belong to different categories within the general taxonomy of error correction, they share the characteristic of being tailored to work efficiently on very specific physical layouts.

\myparagraph{Heavy-Hexagon Code}
A notable example of an architecture-specific code is the heavy-hexagon code, which was designed to operate on a heavy-hexagon lattice topology and introduced as a sparse alternative to the surface code \cite{Chamberland_2020}. It combines properties of topological codes, as it is encoded on a certain lattice topology, and of subsystem stabilizer codes, as it uses gauge operators to reduce the required qubit connectivity to 3. Its qualities make it particularly well-suited for the IBM’s quantum devices with heavy-hex topology, such as IBM Heron \cite{AbuGhanem_2025}.
%Note that the distance $d$ for the HH Code is odd for performance reasons (similar to the surface code) \cite{Chamberland_2020}.

%
%\begin{figure}[ht]
%    \centering
%    \begin{minipage}[t]{0.48\textwidth}
%        \centering
%        \input{figures/taxonomy_venn}
%        \caption{Venn diagram presenting overlap of the dominant families of subsystem quantum error %correction codes.}
 %       \label{fig:taxonomy_venn}
 %   \end{minipage}
 %   \hfill
 %   \begin{minipage}[t]{0.48\textwidth}
 %       \centering
 %       \input{figures/scope_spiderchart}
 %       \caption{Problem dimensions covered in the scope of this project and the level of coverage}
 %       \label{fig:axes}
 %   \end{minipage}
%\end{figure}

%\input{tables/taxonomy_table}
