# Supplementary material for: ECCentric: An Empirical Analysis of Quantum Error Correction Codes
Source: arXiv:2511.01062 source file (2026-08-18)
Supplement: Supplementary file 5 [file appendix.tex]

%\appendix
%\input{appendix_sections/experiments}
