# Supplementary material for: ECCentric: An Empirical Analysis of Quantum Error Correction Codes
Source: arXiv:2511.01062 source file (2026-08-18)
Supplement: Supplementary file 6 [file revisions.tex]

\section{Revision Summary}


\noindent
As part of the resubmission process, we provide this section to outline the improvements we have made in response to the reviewer's comments. We structure it around the \textbf{major comments (M)}, \textbf{the reviewers' comments (A-C)}, and \textbf{our own comments (O)}. ``New exp.'' denotes new experiments. Changed text and figures are marked in blue.

\input{tables/revisions}
